# Supplementary material for: The Phone Walkers: A study of human dependence on inactive mobile devices
Source: arXiv:1804.08753 source file (2018-04-23)
Supplement: Supplementary file 1 [file Appendix.pdf]

# Appendix

We dedicate this appendix to display different tables of the data collected for the study, and their statistical analysis.

## A. Data collection

| Data Set # | Neigbourhood | Day of the Week | Time start | Total Women | Total Men | Total People |
|---|---|---|---|---|---|---|
| 1 | St Germain/Paris | Saturday | 18:12 | 220 | 162 | 382 |
| 2 | Metro Arts t metiers | Sunday | 14:55 | 178 | 187 | 365 |
| 3 | Montorgueil | Sunday | 18:00 | 275 | 258 | 533 |
| 4 | Montorgueil | Sunday | 18:30 | 367 | 386 | 753 |
| 5 | Marias | Monday | 11:00 | 133 | 102 | 235 |
| 6 | Place monge | Monday | 13:00 | 122 | 133 | 255 |
| 7 | Ecoles | Moday | 15:00 | 241 | 134 | 375 |
| 8 | Ecoles | Moday | 14:30 | 97 | 43 | 140 |

**Table A.1.** Sample details and total people observed in each sample.

| Data Set # | Neigbourhood | Day of the Week | Time start | Total Women | Total Men | Total People | Total pairs | Total single sex pairs | Total mixed pairs | Total groups |
|---|---|---|---|---|---|---|---|---|---|---|
| 1 | St Germain/Paris | Saturday | 18:12 | 220 | 162 | 382 | 126 | 43 | 83 | 256 |
| 2 | Metro Arts t metiers | Sunday | 14:55 | 178 | 187 | 365 | 101 | 23 | 78 | 264 |
| 3 | Montorgueil | Sunday | 18:00 | 275 | 258 | 533 | 173 | 62 | 111 | 360 |
| 4 | Montorgueil | Sunday | 18:30 | 367 | 386 | 753 | 250 | 85 | 165 | 503 |
| 5 | Marias | Monday | 11:00 | 133 | 102 | 235 | 48 | 23 | 25 | 187 |
| 6 | Place monge | Monday | 13:00 | 122 | 133 | 255 | 63 | 31 | 32 | 192 |
| 7 | Ecoles | Moday | 15:00 | 241 | 134 | 375 | 52 | 34 | 18 | 323 |
| 8 | Ecoles | Moday | 14:30 | 97 | 43 | 140 | 16 | 9 | 7 | 124 |
| | Totals | | | 1633 | 1405 | 3038 | 829 | 310 | 519 | 2209 |

**Table A.2.** Total single walkers and pairs observed in each sample.

| Data Set # | Total pairs | Total single sex pairs | Total mixed pairs | Total groups |
|---|---|---|---|---|
| 1 | 126 | 43 | 83 | 256 |
| 2 | 101 | 23 | 78 | 264 |
| 3 | 173 | 62 | 111 | 360 |
| 4 | 250 | 85 | 165 | 503 |
| 5 | 48 | 23 | 25 | 187 |
| 6 | 63 | 31 | 32 | 192 |
| 7 | 52 | 34 | 18 | 323 |
| 8 | 16 | 9 | 7 | 124 |
| Totals | 829 | 310 | 519 | 2209 |

**Table A.3.** Distribution of pairs observed in each sample.

| Data Set # | Total single sex pairs | Total mixed pairs | Total groups | Total single sex groups | Total single sex women | Total single sex men |
|---|---|---|---|---|---|---|
| 1 | 43 | 83 | 256 | 173 | 108 | 65 |
| 2 | 23 | 78 | 264 | 186 | 83 | 103 |
| 3 | 62 | 111 | 360 | 249 | 125 | 124 |
| 4 | 85 | 165 | 503 | 338 | 157 | 181 |
| 5 | 23 | 25 | 187 | 162 | 90 | 72 |
| 6 | 31 | 32 | 192 | 160 | 77 | 83 |
| 7 | 34 | 18 | 323 | 305 | 199 | 106 |
| 8 | 9 | 7 | 124 | 117 | 83 | 34 |
| Totals | 310 | 519 | 2209 | 1690 | 922 | 768 |

**Table A.4.** Distribution of walkers by gender observed in each sample.

## B. Phone Walkers

| Data Set # | Women Alone Total | Men Alone Total | Women Alone With Phone | Men Alone With Phone | Women Alone Not with Phone | Men Alone Not with Phone |
|---|---|---|---|---|---|---|
| 1 | 79 | 51 | 31 | 18 | 48 | 33 |
| 2 | 66 | 97 | 20 | 30 | 46 | 67 |
| 3 | 86 | 101 | 32 | 31 | 54 | 70 |
| 4 | 112 | 141 | 37 | 44 | 75 | 97 |
| 5 | 72 | 67 | 27 | 20 | 45 | 47 |
| 6 | 64 | 65 | 20 | 15 | 44 | 50 |
| 7 | 175 | 96 | 76 | 33 | 99 | 63 |
| 8 | 76 | 32 | 34 | 9 | 42 | 23 |
| Totals | 730 | 650 | 277 | 200 | 453 | 450 |

**Table B.1.** Distribution of single walkers and whether they were phone walkers observed in each sample.

| Data # | 1 Man | 1 Woman | 2 Men | 2 Women | 2 Mixed |
|---|---|---|---|---|---|
| 1 | 35.29 | 39.24 | 21.43 | 37.93 | 7.23 |
| 2 | 30.93 | 30.3 | 16.67 | 41.18 | 15.38 |
| 3 | 30.69 | 37.21 | 34.78 | 28.21 | 17.12 |
| 4 | 31.2 | 33.03 | 20 | 22.22 | 12.73 |
| 5 | 29.85 | 37.5 | 20 | 33.33 | 20 |
| 6 | 23.08 | 31.25 | 27.78 | 38.46 | 34.37 |
| 7 | 34.37 | 43.43 | 30 | 50 | 22.22 |
| 8 | 28.12 | 44.74 | 0 | 71.43 | 0 |

**Table B.2.** Percentages of phone walkers by group size observed in each sample.

| Data # | Total People | Total Men | Men users | Total Women | Women users | Total People Users |
|---|---|---|---|---|---|---|
| 1 | 382 | 42.41 | 6.02 | 57.59 | 13.09 | 19.11 |
| 2 | 365 | 51.23 | 9.86 | 48.77 | 9.86 | 19.73 |
| 3 | 533 | 48.4 | 9.57 | 51.59 | 10.13 | 19.7 |
| 4 | 753 | 51.26 | 9.16 | 48.74 | 7.17 | 16.33 |
| 5 | 235 | 43.4 | 9.79 | 56.59 | 15.74 | 25.53 |
| 6 | 255 | 52.16 | 10.59 | 47.84 | 12.55 | 23.14 |
| 7 | 375 | 35.73 | 10.67 | 64.27 | 24.53 | 35.2 |
| 8 | 140 | 30.71 | 6.43 | 69.28 | 29.29 | 35.71 |
| Total | 3038 | 46.25 | 9.15 | 53.75 | 13.03 | 22.18 |

**Table B.3.** Percentages of phone walkers by gender observed in each sample.

# C. Standard Errors

| Group | Total Number | % of total in group size | Standard Error |
|---|---|---|---|
| Single Male | 650 | 47.1 | 3.75 |
| Single Female | 730 | 52.9 | 3.75 |
| Two Males | 236 | 14.23 | 2.42 |
| Two Females | 384 | 23.16 | 4.22 |
| Two Mixed | 1038 | 62.6 | 4.93 |
| All Males | 1405 | 46.25 | 2.79 |
| All Females | 1633 | 53.75 | 2.79 |
| All Persons | 3038 | 100 | 67.75 |
| Total Pairs | 829 | 100 | 27.33 |
| Total Singles | 1380 | 100 | 21.32 |

**Table C.1.** Standard errors for people observed by gender and group size.

| Pairs | Total Number | % of total in group size | Standard Error |
|---|---|---|---|
| Male - 0 phone | 89 | 75.42 | 3.73 |
| Male - 1 phone | 25 | 21.19 | 3.03 |
| Male - 2 phones | 4 | 3.39 | 1.29 |
| Total Male pairs | 118 | 100 | 4.38 |
| Female - 0 phone | 125 | 65.1 | 5.33 |
| Female - 1 phone | 52 | 27.08 | 2.99 |
| Female - 2 phones | 15 | 7.81 | 3.01 |
| Total Female pairs | 192 | 100 | 4.6 |
| Mixed - 0 phone | 441 | 84.97 | 3.63 |
| Mixed - 1 phone Male | 41 | 7.9 | 2.21 |
| Mixed - 1 phone Female | 33 | 6.36 | 1.77 |
| Mixed - 1 phone | 74 | 14.26 | 3.36 |
| Mixed - 2 phones | 4 | 0.77 | 0.56 |
| Total Mixed pairs | 519 | 100 | 19.3 |

**Table C.2.** Standard errors for phone walkers in pairs obsessed of each type.

| Single Walkers | Total Number | % of total in group size | Standard Error |
|---|---|---|---|
| Total Male | 690 | 100 | 4.38 |
| Male - 0 phone | 200 | 28.98 | 1.33 |
| Male - 1 phone | 490 | 71.01 | 1.33 |
| Total Female | 730 | 100 | 4.6 |
| Female - 0 phone | 453 | 62.05 | 1.89 |
| Female - 1 phone | 277 | 37.94 | 1.89 |

**Table C.3.** Standard errors for single phone walkers by gender observed.

| In all pairs | Total Number | % of total in group size | Standard Error |
|---|---|---|---|
| Males - 0 phone | 644 | 89.2 | 2.35 |
| Males - Phone Walkers | 78 | 10.8 | 2.35 |
| Total Males | 722 | 100 | 4.38 |
| Females - 0 phone | 743 | 86.2 | 2.97 |
| Females - Phone Walkers | 119 | 13.8 | 2.97 |
| Total Females | 862 | 100 | 4.6 |

**Table C.4.** Standard errors by gender in pairs of phone walkers observed.
